# Supplementary material for: Machine Learning Sensors
Source: arXiv:2206.03266 source file (2022-06-07)
Supplement: Supplementary file 1 [file appendix.tex]

\appendix

\section{Appendix}

% \subsubsection*{Object Counter}

% \subsubsection*{Flow Detector}

% \subsubsection*{Person Recognizer}
